# Supplementary material for: Prediction of a Feshbach Resonance in the Below-the-Barrier Reactive Scattering of Vibrationally Excited HD with H
Source: arXiv:2006.10374 source file (2020-06-18)
Supplement: Supplementary file 1 [file Supporting_Information.pdf]

Supporting Information for

# Prediction of a Feshbach Resonance in the Below-the-Barrier Reactive Scattering of Vibrationally Excited HD with H

Boyi Zhou,[†,‡] Benhui Yang,[†] N. Balakrishnan,[§] B. K. Kendrick,[‖] and P. C. Stancil[*,†]

[†]*Department of Physics and Astronomy and Center for Simulational Physics, University of Georgia, Athens, Georgia 30602, United States*

[‡]*Key Laboratory of Materials Modification by Laser, Electron, and Ion Beams (Ministry of Education), School of Physics, Dalian University of Technology, Dalian 116024, P. R. China*

[§]*Department of Chemistry and Biochemistry, University of Nevada, Las Vegas, Nevada 89154, United States*

[‖]*Theoretical Division (T-1, MS B221), Los Alamos National Laboratory, Los Alamos, New Mexico 87545, United States*

*Corresponding author. Email: pstancil@uga.edu

| **Table S1.** | Parameters in the calculations for the HD + H reaction with the ABC program | | |
|---|---|---|---|
| | E ⩽ 1000 $cm^{-1}$ | E > 1000 $cm^{-1}$ | |
| *jtot* | 0-30 | 0-120 | Total angular momentum quantum number $J$ |
| *ipar* | $(-1)^J$ | $(-1)^J$ | Triatomic parity eigenvalue $P$ |
| *jpar* | 0 | 0 | Diatomic parity eigenvalue $p$ |
| *rmax* | 20 | 15 | Maximum hyperradius $\rho_{max}$ (in bohr) |
| *mtr* | 5000 | 200 | Number of log derivative propagation sectors |
| *jmax* | 15 | 15 | Maximum rotational quantum number of any channel |
| *kmax* | 10 | 10 | Helicity truncation parameter $k_{max}$ |
| *emax* | 2.7 | 2.7 | Maximum internal energy in any channel (in eV) |

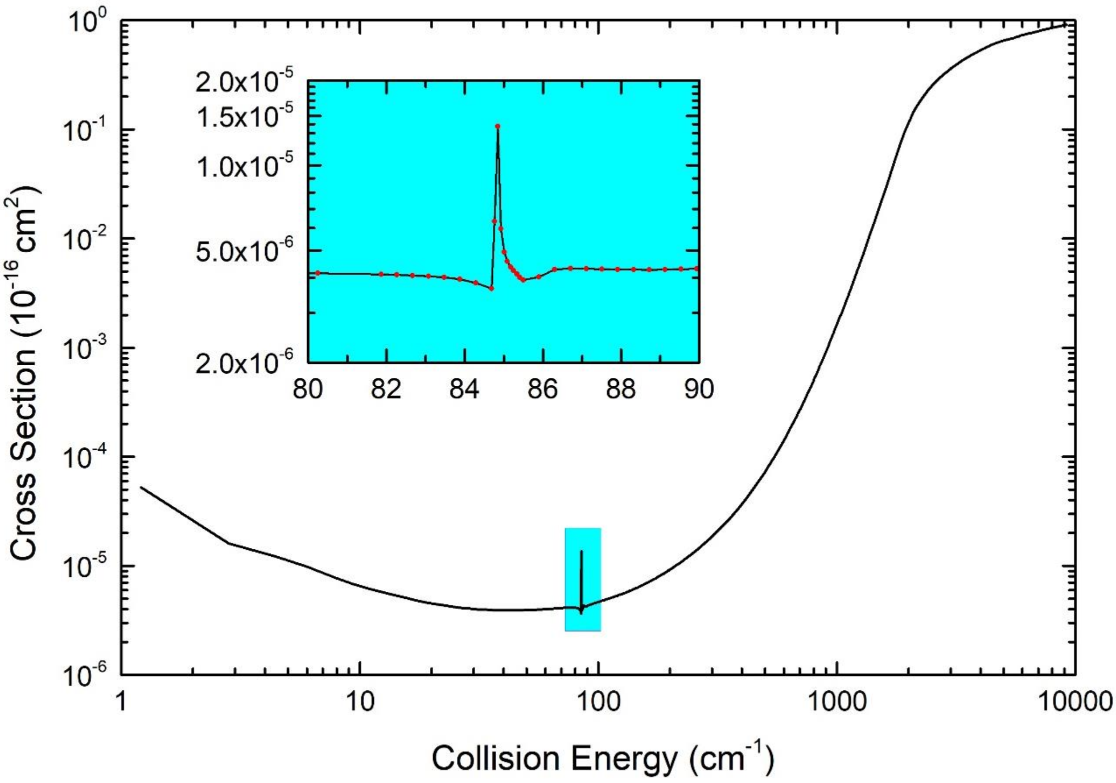


**Figure S1.** Collision energy variation of the cross section for the reactive process (sum over all final states) for the HD ($v$ = 1, $j$ = 0) + H reaction.

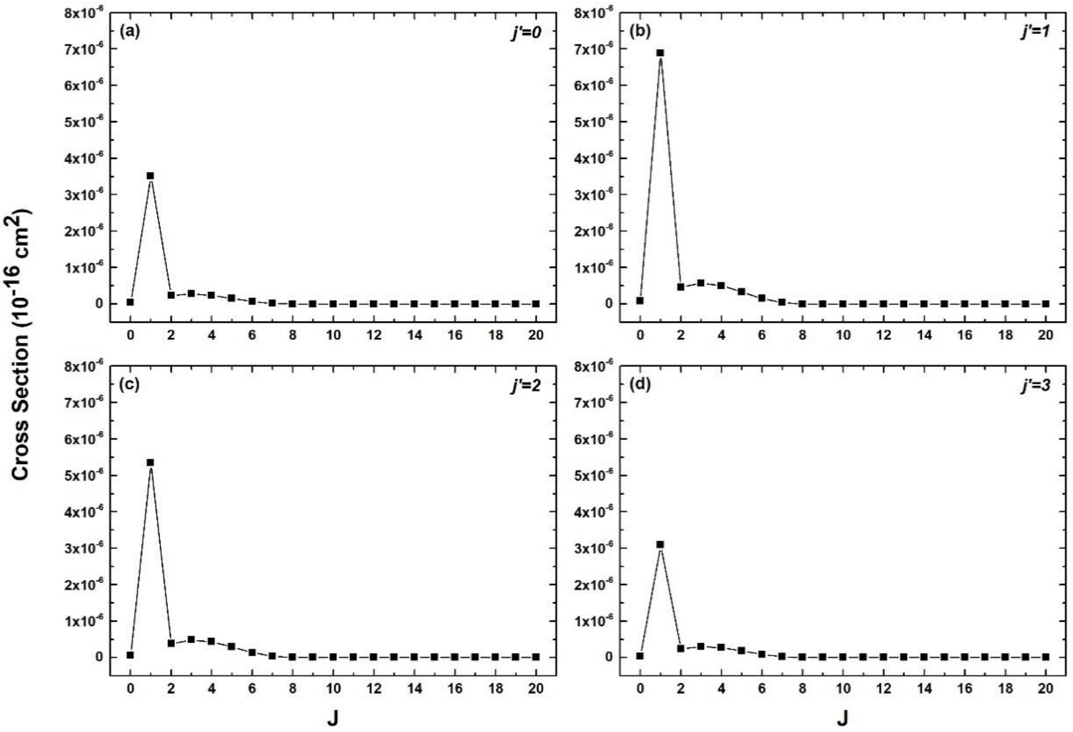


**Figure S2.** Contributions from each $J$ to the cross sections for the HD ($v$ = 1, $j$ = 0) + H → D + $H_2$ ($v'$ = 0, $j'$) reaction with rotational final states (a) $j'$ = 0, (b) $j'$ = 1, (c) $j'$ = 2, (d) $j'$ = 3.

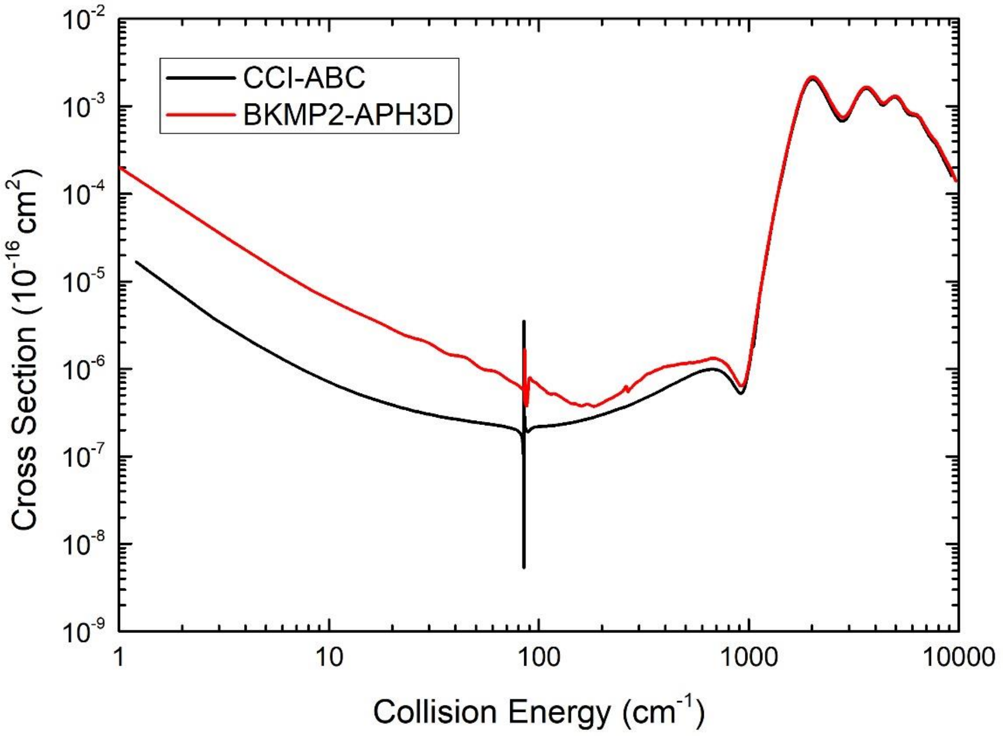


**Figure S3.** A comparison of collision energy variation of the cross section for HD ($v$ = 1, $j$ = 0) + H → D + $H_2$ ($v'$ = 0, $j'$ = 0) reaction on the CCI PES using the ABC program (black line) and on the BKMP2 PES using the APH3D program (red line) for $J$ = 1.

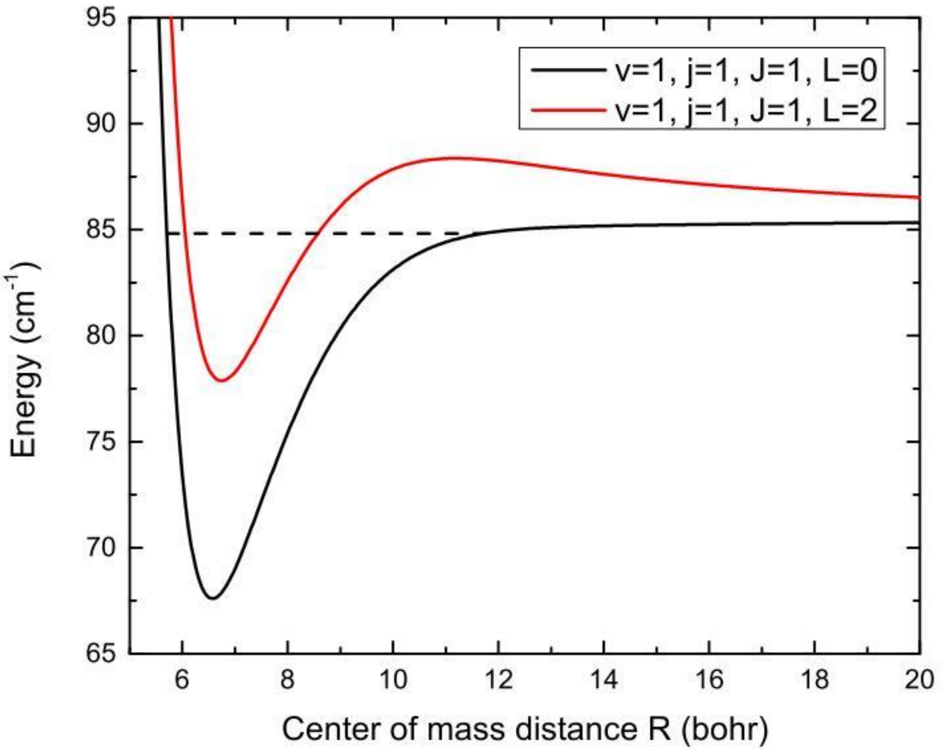


**Figure S4.** Adiabatic potentials correlating with different ($v$, $j$) states of HD in HD ($v$ = 1, $j$ = 0) collisions for $J$ = 1 on the BKMP2 PES.

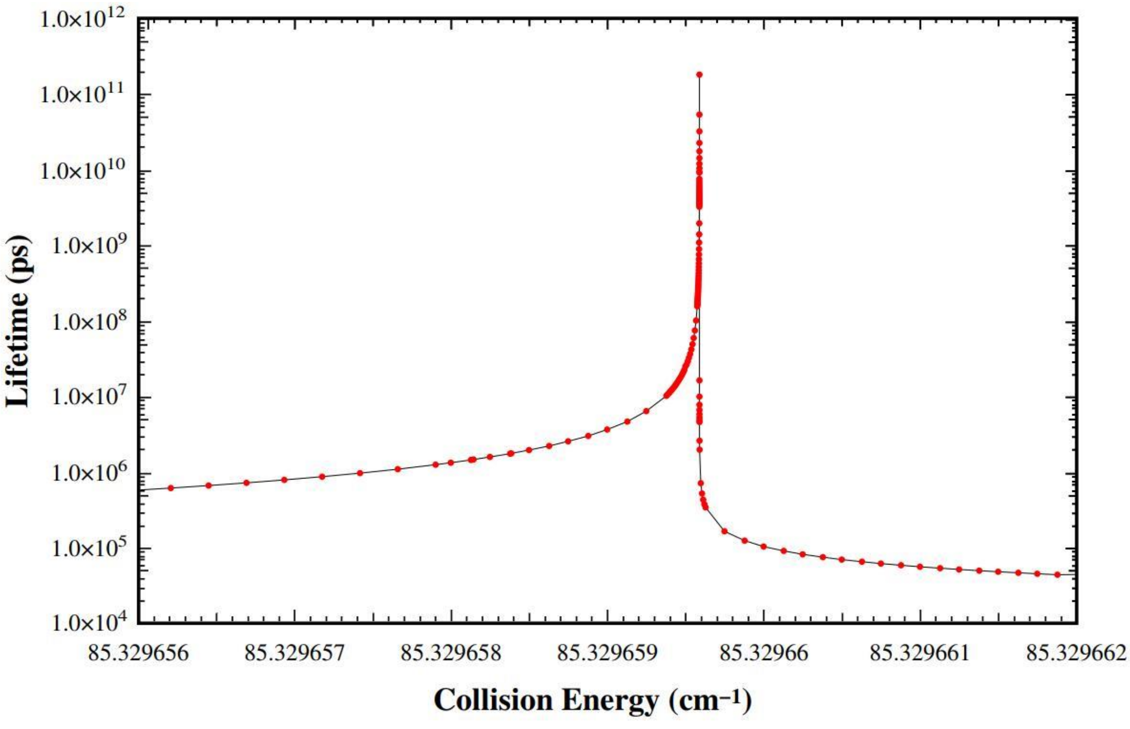


**Figure S5.** Lifetime of the Feshbach resonance in the below-the-barrier reactive scattering of the HD ($v$ = 1, $j$ = 0) + H collision on the BKMP2 PES using the APH3D program for $J$ = 1.

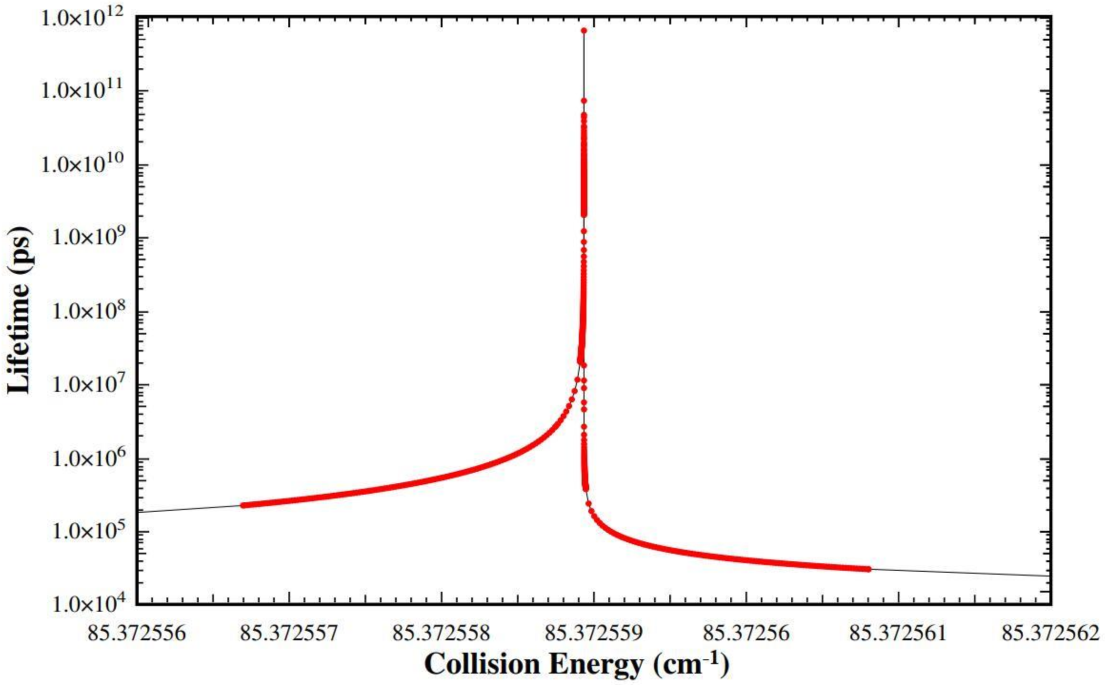


**Figure S6.** Lifetime of the Feshbach resonance in the below-the-barrier reactive scattering of the HD ($v$ = 1, $j$ = 0) + H collision on the CCI PES using the APH3D program for $J$ = 1.
